# Supplementary material for: Measurement of Untruncated Nuclear Spin Interactions via Zero- to Ultra-Low-Field Nuclear Magnetic Resonance
Source: arXiv:1501.05768 source file (2015-10-25)
Supplement: Supplementary file 1 [file RDC_SI_v2.1.pdf]

# Supplemental Material for Measurement of Untruncated Nuclear Spin Interactions via Zero- to Ultra-Low-Field Nuclear Magnetic Resonance

J. W. Blanchard,[1,2,3] T. Sjolander,[1,2] J. P. King,[1,2] M. P. Ledbetter,[4] E. H. Levine,[2] V. S. Bajaj,[1,2] D. Budker,[3,4,5] and A. Pines[1,2]

[1]*Materials Science Division, Lawrence Berkeley National Laboratory, Berkeley, CA, 94720*
[2]*Department of Chemistry, University of California at Berkeley, CA, 94720*
[3]*Helmholtz-Institut Mainz, Johannes Gutenberg University, Germany*
[4]*Department of Physics, University of California at Berkeley, CA, 94720-7300*
[5]*Nuclear Science Division, Lawrence Berkeley National Laboratory, Berkeley, CA, 94720*

(Dated: July 5, 2015)

This document contains supplemental information for the manuscript *Measurement of Untruncated Nuclear Spin Interactions via Zero- to Ultra-Low-Field Nuclear Magnetic Resonance*, including additional details of sample preparation and characterization, along with further elaboration of the first-order perturbation theory presented in the main text and a comparison with exact numerical simulations. We also elaborate on the rotation of the effective detection operator in applied magnetic fields, both in terms of the effect on the nuclear spin system and in terms of the effect on alkali spins in the atomic vapor magnetometer.

## SAMPLE PREPARATION

Polyvinyl acetate (PVAc) polymer sticks containing between 1-6% v/v divinyl adipate (DVA) cross-linker were produced via a modified method based on the approach in Ref. [1]. Polymers were prepared in 5 mm NMR tubes by adding the radical initiator azobisisobutyronitrile (AIBN) to a solution of 60% vinyl acetate and 40% acetone by volume. The presence of the acetone was prompted by synthetic considerations: it was found that performing the polymerization reaction without an additional solvent frequently led to cracks or bubbles in the resulting polymer sticks. Presumably, carrying out the reaction in the presence of acetone allowed the reaction to continue to completion in an essentially solution phase without nonlinear issues related to phase transitions occurring during the reaction. The acetone is then easily removed by evaporation. Samples with varying alignment strength were prepared by adding a variable amount of the cross-linker DVA to the mixture before transfer to standard 5 mm NMR tubes – increased cross-linking was found to correlate with increased alignment. The samples were then heated in an oven at 45°C for 7 days to initiate polymerization via thermal decomposition of AIBN, followed by 2 days at 55°C in order to ensure that the reaction went to completion. Anisotropic gels were prepared by adding acetonitrile-2-$^{13}$C (doped with 5% v/v deuterated acetonitrile) to the tubes and allowing the polymers to swell for 2 weeks.[1]

The sample used for Fig. 3 of the main text was prepared via slightly different means, using a nearly identical procedure but with sample heating performed in a temperature-controlled sand bath. The polymer sticks produced using the sand bath were consistently of high quality (based on the absence of visible bubbles, cracks, or other inhomogeneities), so we suggest that this method is generally preferable for future applications of this work. Acetonitrile-2-$^{13}$C was added to the NMR tube containing the polymer stick and immediately frozen using liquid nitrogen. The sample was then degassed and flame-sealed under vacuum, after which the polymer was allowed to swell and equilibrate at room temperature for two weeks.

[1] After two weeks, successive measurements of the quadrupolar splittings (see next section) showed no increase in order parameter, indicating that the swelling had reached equilibrium.

## PERTURBATION THEORY FOR ZERO-FIELD RESIDUAL DIPOLAR COUPLINGS

In the regime where the dipolar coupling strength is small compared to the $J$-coupling ($D_{jk} \ll J_{jk}$), the residual dipolar couplings may be treated as a perturbation on the $J$-coupling. For acetonitrile-2-$^{13}$C, it is convenient to write the first term of Eq. (1) from the main text as

$$\mathcal{H}^{(0)} = \hbar J_{\mathrm{CH}} \mathbf{K} \cdot \mathbf{S}, \tag{1}$$

where $J_{CH}$ is the one-bond $J$-coupling, $\mathbf{S}$ is the $^{13}$C spin angular momentum, and $\mathbf{K} = \sum_j \mathbf{I}_j - \mathbf{S}$ is the total proton spin angular momentum [2]. The eigenstates of $\mathcal{H}^{(0)}$ are also eigenstates of $\mathbf{F}^2$ and $F_z$, where $\mathbf{F} = \mathbf{K} + \mathbf{S}$ is the total spin angular momentum. The eigenstates have degeneracy $2F + 1$ and energy

$$E^{(0)} = \frac{\hbar J_{\mathrm{CH}}}{2} \left[ F(F+1) - K(K+1) - S(S+1) \right]. \tag{2}$$

To explore the effect of the residual dipolar coupling on the $J$-coupling eigenstates, it is convenient to decompose Eq. (2) from the main text into two heteronuclear terms,

$$\mathcal{H}^{(1a)} = -3\hbar D_{\mathrm{CH}} K_z S_z \tag{3}$$

and

$$\mathcal{H}^{(1b)} = \hbar D_{\mathrm{CH}} \mathbf{K} \cdot \mathbf{S}, \tag{4}$$

where $D_{CH}$ is the dipolar coupling strength between $^{13}$C and $^{1}$H spins, and a homonuclear term,

$$\mathcal{H}^{(1c)} = -\hbar D_{HH} \sum_{j;k>j}^{3} \left(3 I_{j,z} I_{k,z} - \mathbf{I}_j \cdot \mathbf{I}_k\right), \quad (5)$$

where $D_{HH}$ is the dipolar coupling strength between $^{1}$H spins, and where the sum is limited to $^{1}$H spins.

To first order in $D_{CH}$, the energy shifts due to the heteronuclear residual dipolar coupling are

$$\begin{aligned}\Delta E^{(1a)} &= -3\hbar D_{CH} \langle F m_F | K_z S_z | F m_F \rangle \\ &= -3\hbar D_{CH} \sum_{m_K, m_S} \langle K S m_K m_S | F m_F \rangle^2 m_K m_S, \end{aligned} \quad (6)$$

where $\langle K S m_K m_S | F m_F \rangle$ are the Clebsch-Gordan coefficients, and

$$\begin{aligned}\Delta E^{(1b)} &= \hbar \frac{D_{CH}}{2} \langle F m_F | \left(\mathbf{F}^2 - \mathbf{K}^2 - \mathbf{S}^2\right) | F m_F \rangle \\ &= \hbar \frac{D_{CH}}{2} \left[ F(F+1) - K(K+1) - \frac{3}{4} \right]. \end{aligned} \quad (7)$$

For all $K = \frac{1}{2}$ states, the homonuclear residual dipolar coupling has no effect, as the rank-2 spherical-tensor operator of Eq. (5) defined in terms of proton angular momentum can only connect two states having total proton angular momentum $K$ and $K'$ such that $K + K' \geq 2$. The total energy shifts for the $K = \frac{1}{2}$ states are thus

$$\Delta E^{(1)}\left(F = 0, m_f = 0\right) = 0, \quad (8)$$

$$\Delta E^{(1)}\left(F = 1, m_f = 0\right) = \hbar D_{CH}, \quad (9)$$

$$\Delta E^{(1)}\left(F = 1, m_f = \pm 1\right) = -\frac{\hbar}{2} D_{CH}. \quad (10)$$

The first-order energy shifts due to the homonuclear residual dipolar couplings for the $K = \frac{3}{2}$ may be calculated in a similar method to that of Eqs. (6) and (7), though the effects of couplings between equivalent spins must be considered. An analytical derivation of these shifts requires either the use of 9-j symbols or a long string of Clebsch-Gordan coefficients, so it is generally more convenient to calculate the shifts using symbolic matrix multiplication in software such as Mathematica (Wolfram Research, Inc.). The total shifts for the $K = \frac{3}{2}$ states are

$$\Delta E^{(1)}\left(F = 1, m_F = 0\right) = -\frac{\hbar}{2}\left(D_{CH} - 3D_{HH}\right), \quad (11)$$

$$\Delta E^{(1)}\left(F = 1, m_F = \pm 1\right) = \frac{\hbar}{4}\left(D_{CH} - 3D_{HH}\right), \quad (12)$$

$$\Delta E^{(1)}\left(F = 2, m_F = 0\right) = \frac{3\hbar}{2}\left(D_{CH} + D_{HH}\right), \quad (13)$$

$$\Delta E^{(1)}\left(F = 2, m_F = \pm 1\right) = \frac{3\hbar}{4}\left(D_{CH} + D_{HH}\right), \quad (14)$$

$$\Delta E^{(1)}\left(F = 2, m_F = \pm 2\right) = -\frac{3\hbar}{2}\left(D_{CH} + D_{HH}\right). \quad (15)$$

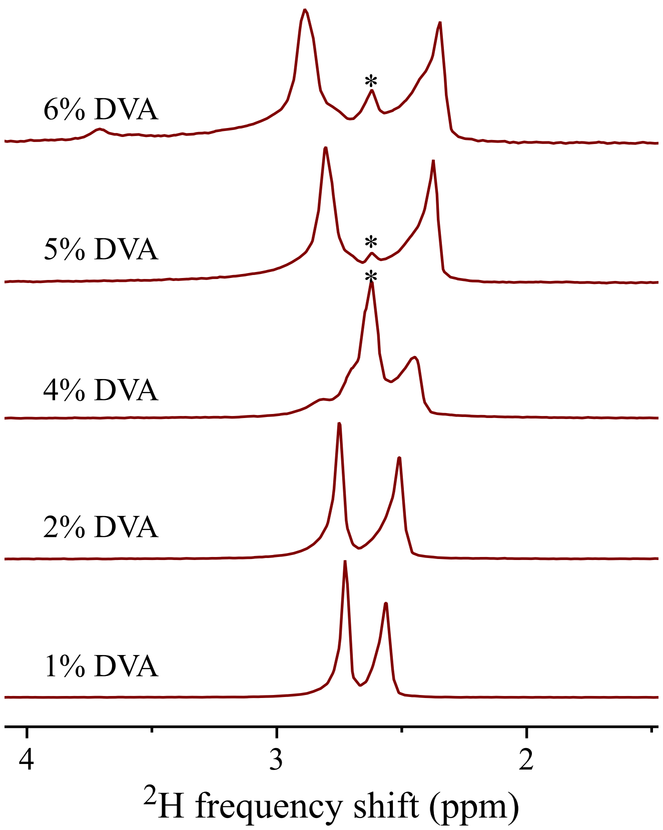


FIG. 1. $^{2}$H quadrupolar splittings of acetonitrile-d$_3$ measured at high field for swollen PVAc gels with different degree of alignment arising from the concentration of the cross-linker divinyl adipate (DVA). Isotropic peaks due to inhomogeneous regions in the gels are denoted by an asterisk.

## HIGH-FIELD $^{2}$H QUADRUPOLE SPLITTINGS

The deuterium nucleus is a spin-1 particle and thus interacts with electric field gradients via its quadrupole moment. The first-order Hamiltonian for this interaction in aligned samples at high-field can be written as [3]

$$H = S_{zz} \frac{e^2 q_{zz} Q}{4I(2I-1)} \left(3 I_z I_z - \mathbf{I} \cdot \mathbf{I}\right), \quad (16)$$

where $S_{zz}$ is the molecular order parameter, $e$ is the electric charge, $eq_{zz}$ is the $zz$ element of the electric field gradient (EFG) tensor, $Q$ is the nuclear quadrupole moment, and $\mathbf{I}$ is the nuclear angular momentum operator. The interaction in Eq. (16) splits the $^{2}$H NMR resonance into two lines separated by

$$\Delta\nu = \frac{3}{2} S_{zz} e^2 q_{zz} Q / h. \quad (17)$$

Equation (17) implies that if the value of the EFG along the $z$ axis in the molecular frame ($C_3$ axis in acetonitrile) is known then the molecular order parameter for a given sample can be determined directly from the $^{2}$H high-field NMR spectrum

[4]. The value for the EFG in $CD_3CN$ has been determined previously such that $e^2 q_{zz} Q/h = 54.5$ Hz [4].

Figure 1 shows $^2$H quadrupolar splittings of acetonitrile-$d_3$ for the samples in a 14.1 T NMR spectrometer with deuterium frequency 92.1 MHz. Each spectrum consists of a doublet corresponding to partially ordered acetonitrile and a central isotropic peak (marked with an asterisk) originating from acetonitrile external to the gel. Because the $^2$H spectrum for the sample containing 4% DVA cross-linker is notably more complicated than the other spectra, it may not be immediately apparent how to extract the appropriate quadrupolar splitting. It was determined that the complexity of the $^2$H spectrum for the 4% DVA sample was due to inhomogeneities in the gel on the length scale of the high-field detection coil. Varying the vertical position of the sample in the coil showed that the peaks corresponding to the gel near the bottom of the sample tube (the region to which the zero-field detector is most sensitive) are the left- and rightmost peaks of the 4% DVA spectrum. The following values for the splittings in each spectrum were extracted using the Mestrenova software package (Mestrelab Research Inc.): 14.6 Hz (1% DVA), 21.9 Hz (2% DVA), 32.4 Hz (4% DVA), 39.6 Hz (5% DVA) and 49.7 Hz (6% DVA). Using Eq. (17) these splittings were converted into values for the molecular order parameter for each sample prior to the zero field experiments. The resulting measured molecular order parameters are $1.79 \times 10^{-4}$ (1% DVA), $2.68 \times 10^{-4}$ (2% DVA), $3.96 \times 10^{-4}$ (4% DVA), $4.84 \times 10^{-4}$ (5% DVA), and $6.08 \times 10^{-4}$ (6% DVA).

## COMPARISON OF 1ST ORDER PERTURBATION THEORY AND EXACT NUMERICAL SIMULATIONS

The predicted transition frequencies in aligned 2-$^{13}$C-acetonitrile at zero magnetic field are shown in Fig. 2 as a function of molecular order parameter. The solid black lines are computed by an exact numerical simulation, and the dashed red lines are calculated from the equations in the main text, derived from first-order perturbation theory. For order parameters in the range of $0 - 10^{-3}$, there is no resolvable difference between the values predicted by first-order perturbation theory and those predicted by the exact numerical simulation.

## ROTATION OF EFFECTIVE DETECTION OPERATOR IN APPLIED MAGNETIC FIELDS

Figure 3 shows simulated spectra (obtained by numerical propagation of the density matrix) for the $K = 1/2$ peaks of acetonitrile-2-$^{13}$C aligned in stretched PVAc gels as a function of magnetic field applied orthogonal to the director axis. The simulation only shows the effect of the magnetic field on the nuclear spins (i.e. the mixing of states with different $m_F$), leading to the appearance of nominally forbidden $\Delta m_F = \pm 1$ transitions. Such effects partially contribute to the observed

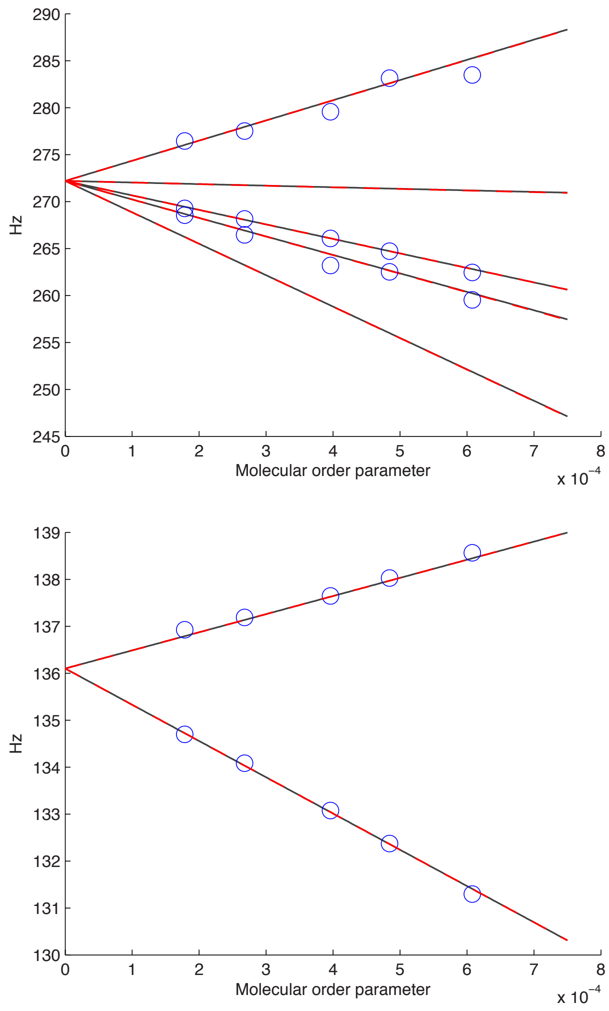


FIG. 2. Transition frequencies between $K = \frac{3}{2}$ states (top) and between $K = \frac{1}{2}$ states (bottom) in aligned 2-$^{13}$C-acetonitrile as a function of molecular order parameter from first-order perturbation theory (dashed lines) and exact numerical simulation (solid lines). Within this range of order parameter, the predictions of first-order perturbation theory are indistinguishable from the exact numerical simulation.

increase in the $\Delta m_F = \pm 1$ transition, but are insufficient to explain the full change in the effective detection operator.

The remaining effect is likely due to the rotation of the sensitive axis of the magnetometer by the applied magnetic field. In general, our measurement is sensitive to the alkali spin polarization in the $x$ direction. The overall equation for the evolution of the atomic spin, $\boldsymbol{S}_a$, may be written as

$$\frac{\mathrm{d}}{\mathrm{d}t}\boldsymbol{S}_a = \frac{1}{2I+1}\left[\frac{g_s \mu_B}{\hbar}\boldsymbol{B} \times \boldsymbol{S}_a + R_{OP}\left(\frac{1}{2}s\hat{\boldsymbol{y}} - \boldsymbol{S}_a\right) - R_{rel}\boldsymbol{S}_a\right], \tag{18}$$

where $I$ is the nuclear spin, $g_s$ is the atomic $g$-factor, $\mu_B$ is the Bohr magneton, and including the competing effects of optical pumping along the pumping axis ($y$), $R_{OP}$, spin relaxation randomizing the spin direction, $R_{rel}$, and spin precession induced

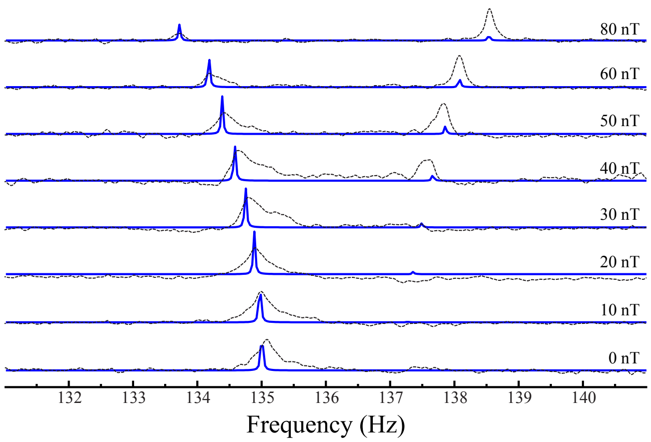


FIG. 3. Simulations showing the appearance of nominally forbidden transitions as a consequence of adding an external field, including only the effect on nuclear spins (neglecting the effect on the magnetometer sensitivity). Simulations are solid blue lines, and experimental data are shown with dashed lines for comparison. Simulated spectra are shown with a narrow linewidth for clarity.

by the magnetic field [5].

In the absence of a magnetic field, the equilibrium spin polarization is

$$S_{a,0} = \frac{sR_{\mathrm{OP}}}{2\left(R_{\mathrm{OP}} + R_{\mathrm{rel}}\right)}. \tag{19}$$

In the limit of slowly varying magnetic fields, $\mathrm{d}\boldsymbol{S}_a/\mathrm{d}t \rightarrow 0$, and the steady state solution of Eq. (18) yields the following components of the spin:

$$S_{a,x} = S_{a,0}\frac{\beta_z + \beta_x\beta_y}{1 + \beta_x^2 + \beta_y^2 + \beta_z^2}, \tag{20}$$

where

$$\boldsymbol{\beta} = \left[\frac{g_s\mu_{\mathrm{B}}}{\hbar(R_{\mathrm{OP}} + R_{\mathrm{rel}})}\right]\boldsymbol{B}. \tag{21}$$

Based on Eq. (20), the magnetometer should, to first order, be sensitive only to fields in the $z$ direction, unless an additional static field is applied. Application of a static magnetic field in the pump direction ($y$) leads to increased sensitivity to fields in the $x$ direction. This may be interpreted as a rotation of the effective detection operator.

[1] J. C. Freudenberger, S. Knör, K. Kobzar, D. Heckmann, T. Paululat, H. Kessler, and B. Luy, Angewandte Chemie **117**, 427 (2005).
[2] M. P. Ledbetter, T. Theis, J. W. Blanchard, H. Ring, P. Ganssle, S. Appelt, B. Blümich, A. Pines, and D. Budker, Phys. Rev. Lett. **107**, 107601 (2011).
[3] C. P. Slichter, *Principles of Magnetic Resonance* (Springer, 1990), 3rd ed.
[4] W. J. Caspary, F. Millett, M. Reichbach, and B. P. Dailey, J. Chem. Phys. **51**, 623 (1969).
[5] S. Seltzer and M. Romalis, Appl. Phys. Lett. **85**, 4804 (2004).
